# Supplementary material for: MambaPEFT: Exploring Parameter-Efficient Fine-Tuning for Mamba
Source: arXiv:2411.03855 source file (2025-04-01)
Supplement: Supplementary file 1 [file ablation_additional.tex]

\documentclass{standalone}
\usepackage{pgfplots}
\pgfplotsset{compat=1.18}

\begin{document}

% Line plot for AdditionalScan
\begin{tikzpicture}
    \begin{axis}[
        xlabel={Additional dimension},
        ylabel={Acc. (\%)},
        grid=major,
        width=9cm,
        height=6cm,
        legend style={at={(0.5,-0.25)}, anchor=north, legend columns=2},
    ]
    % Top (S4D init)
    \addplot[
        color=blue,
        mark=*,
        line width=1pt,
        ]
        coordinates {
        (1,55.44208333)
        (2,56.7511)
        (4,57.75113333)
        (6,57.5609)
        (8,57.47755)
        };
    \addlegendentry{Top (S4D init)}

    % Top (our init)
    \addplot[
        color=red,
        mark=square*,
        line width=1pt,
        ]
        coordinates {
        (1,59.60426667)
        (2,60.88533333)
        (4,61.30353333)
        (6,61.61215)
        (8,61.36388333)
        };
    \addlegendentry{Top (our init)}

    % Bottom (S4D init)
    \addplot[
        color=green,
        mark=triangle*,
        line width=1pt,
        ]
        coordinates {
        (1,55.39605)
        (2,56.82806667)
        (4,57.30345)
        (6,57.38683333)
        (8,57.93086667)
        };
    \addlegendentry{Bottom (S4D init)}

    % Bottom (our init)
    \addplot[
        color=purple,
        mark=diamond*,
        line width=1pt,
        ]
        coordinates {
        (1,56.30661667)
        (2,60.84046667)
        (4,61.32205)
        (6,61.46273333)
        (8,61.34745)
        };
    \addlegendentry{Bottom (our init)}

    \end{axis}
\end{tikzpicture}

\end{document}
